# Supplementary material for: Bismuth based Half Heusler Alloys with giant thermoelectric figure of merit
Source: arXiv:1610.06038 source file (2016-10-20)
Supplement: Supplementary file 1 [file supplimentary_info.pdf]

# Supporting Information

## Bismuth based Half Heusler Alloys with giant thermoelectric figure of merit

*Vikram, Jiban Kangsabanik, Enamullah and Aftab Alam**

PACS numbers: 31.15.A-, 72.20.Pa, 84.60.Rb, 63.20.kd, 61.72.-y

Here we provide further details on (i) the calculation of formation energy and elastic properties (section 1) (ii) comparison of our theoretical results with a well studied half heusler alloys, namely ZrNiSn (section 2) (iii) phonon properties of the concerned system i.e. HfRhBi, ZrIrBi and ZrRhBi (section 3)

### Section 1

### Formulae for calculation of formation energy and elastic properties: -

The formation energy $\Delta E_F$ with respect to the elemental stable phase is calculated using the following formula,

$$\Delta E_F = E_{tot} - \sum_i w_i \mu_i \qquad (1)$$

Where, $E_{tot}$ is the total energy of alloy per atom, $w_i$ is the weight factor and $\mu_i$ corresponds to the chemical potential of each constituent element in the alloy that represents the total energy per atom in its bulk equilibrium state. Here bulk Hf and Zr are in hcp, Rh and Ir in fcc and Bi in monoclinic phase.

Mechanical stability of the materials is an important property to be assess their thermo electrics. A material with high values of elastic modulus can be subjected to various stresses without changing its properties significantly. In addition to the chemical stability, the mechanical stability of the present alloys (space group F-43m) has also been checked by satisfying the well-known Born-Huang criteria **[1]** involving the elastic constants $(C_{ij})$, given by the following relations,

$$\frac{C_{11} - C_{12}}{2} > 0, \frac{(C_{11} + 2C_{12})}{3} > 0, C_{44} > 0 \qquad (2)$$

The bounds on the values of bulk modulus (B) and shear modulus (G) was originally given by Reuss **[2]** and Voight **[3]** which was later improved by Hashin and Shtrikman **[4]** for cubic crystals. The bulk modulus and Young's modulus (Y) are calculated using the following formulae, **[5]**

$$B = \frac{1}{3}(C_{11} + 2C_{12}) \qquad (3)$$

$G_1 = \frac{1}{2}(C_{11} - C_{22})$ and $G_2 = C_{44}$ where $G_1$ and $G_2$ are the upper (whichever is larger) and lower bound of the shear modulus G.

$$G = \frac{G_1 + G_2}{2} \quad , \quad Y = \frac{9BG}{3B + G} \qquad (4)$$

## Section 2

## Validation of Computational procedure: comparison with ZrNiSn: -

In order to validate our calculation procedure and gain more confidence on the predictability power for the new systems studied here, we performed a thorough *ab-initio* calculation for pure ZrNiSn, which is the most widely studied material for the thermoelectric properties in the half-heusler family. In this section we present a fair comparison of our results with some of the available data as can be seen in Table S.1.

| T = 773 K & $n_c$ = 0.86x$10^{20}$ $cm^{-3}$ | $S(\mu V K^{-1})$ | $\sigma(\Omega^{-1} m^{-1})$ | ZT |
|---|---|---|---|
| Experiment [6] | -266 | 4.5x$10^4$ | ~0.45 |
| Our results | -278 | 4.7x$10^4$ | 0.30 |

***Table S1*** *: Comparison of our theoretically calculation Seebeck coefficient, electrical conductivity and the figure of merit with experiment [6] for n-type ZrNiSn at carrier concentration* $n_c$*=0.86x*$10^{20}$ $cm^{-3}$ *and temperature T=773 K.*

Table S.1 presents a comparison of our theoretical result with the experiment [6] on the Seebeck coefficient (S), electrical conductivity ($\sigma$) and the figure of merit (ZT) for n-type ZrNiSn at a carrier concentration $n_c$ 0.8686x$10^{20}$ $cm^{-3}$ and temperature 773 K. One can notice that S and $\sigma$ agrees fairly well. There is of course some noticeable difference in the ZT values. This difference is attributed to the presence of intrinsic defects, imperfections in the measured sample which usually occur during sample preparation, and which certainly changes the carrier concentration. Our theoretical results, however, are for 100% pure and dense sample. This can be one of the reasons for different optimal values of $n_c$.

However according to our calculation there is another optimal carrier concentration ($n_c$=3.61x$10^{20}$ $cm^{-3}$) which corresponds to maxima in the ZT-value instead of $S^2\,\sigma$. These ZT values are 0.32 at 773K and even higher (0.36) at 1150 K. We also found that there is an optimal p-type carrier concentration ($n_c$=9.03x$10^{20}$ $cm^{-3}$) in which ZT is coming out to be even higher (0.38) at 1150K.

We also compared our calculated lattice thermal conductivity ($\kappa_L$) with available experimental data **[7].** Figure S1 shows a comparison of our calculated $\kappa_L$ with experimentally available data for levitation melted (LM) coarse grained sample and melt-spun (MS) submicron grain size sample of pure ZrNiSn **[7]**. It is clear from the figure that when we use a 2x2x2 supercell with up to $2^{nd}$ nearest neighbour interactions only to calculate the force constants, the calculated $\kappa_L$ does not compare well. However, a 4x4x4 supercell which include $4^{th}$ nearest neighbour interaction in the force constants calculation, gives a much better comparison with experiment.

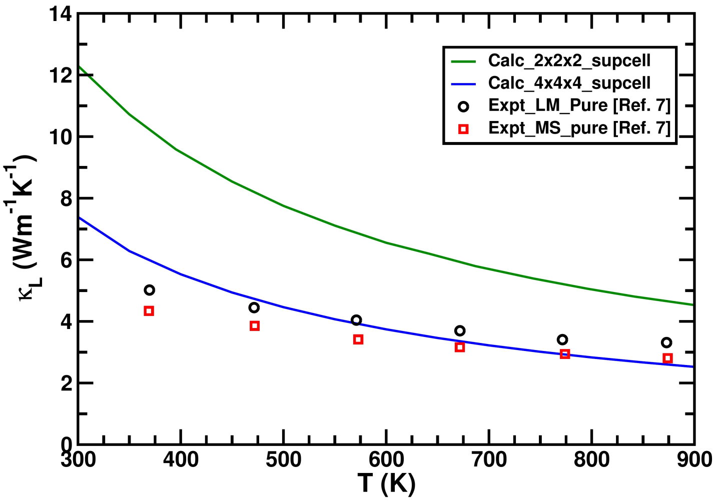


***Figure S1 :*** *Comparison of our calculated lattice thermal conductivity for ZrniSn with the available experimental data [7]. LM stands for levitation melted coarse grained sample and MS for melt-spun submicron grain size sample of pure ZrNiSn*

## Section 3

## Phonon properties of XYBi (X=Hf, Zr; Y=Rh, Ir): -

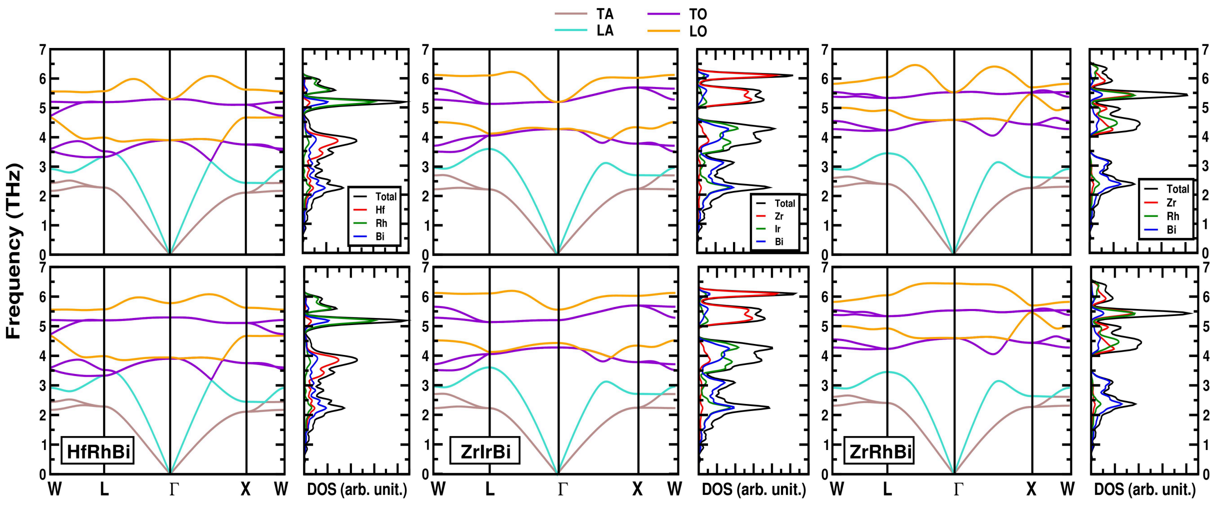


***Figure S2****: Phonon dispersion and phonon density of states by applying LO-TO correction (bottom) and without LO-TO correction (top) for HfRhBi (left), ZrIrBi (center) and ZrRhBi (right)*

Figure S2 shows the phonon density of states and phonon dispersion curves along the high symmetry lines for the three systems. The three atoms give rise to nine phonon branches, i.e., one longitudinal acoustic (LA) mode, two transverse acoustic (TA) modes, two longitudinal optical (LO) modes, and four transverse optical (TO) modes. The two TA modes along the Γ-L and Γ-X directions are two-fold degenerate.

Due to displacement of charges of long-wavelength LO modes, internal electric dipoles are produced which leads to internal electric field. The phonon frequencies for the LO modes at the Γ point shift up due to this induced electric field. Thus, the LO-TO splitting is an important parameter to evaluate the strength of ionicity. The phonon dispersion curves and DOS shown in Figure S1 have both the plots, namely with (below) and without (above) including the LO-TO splitting.

Clearly, the phonon dispersion (below) for the three systems show LO-TO splitting at the Γ point, which implies the existence of the ionic bonding in crystal (more the splitting, more the ionic character). As can be seen from the figure, ZrRhBi has the maximum LO-TO splitting, suggesting it to have the highest ionic character.

Looking at the phonon DOS for HfRhBi, it is seen that the low-frequency branches up to 3 THz are mainly from the Bi atomic vibrations, while the frequency branches between 3 THz and 4.5 THz are mainly from the Hf atomic vibrations. The Rh atomic vibrations contribute to the high-frequency branches above ~4.8 THz. This is due to the difference in masses of the three elements. Rh being the lightest (mass=102.9 amu) vibrating at highest frequencies and Bi being heaviest (mass=208.98) vibrates at the lowest frequencies. The acoustic and optical branches overlap near the L point and between Γ-X direction for HfRhBi due to the comparable masses of the three elements.

For ZrIrBi, Ir (mass=192.22 amu) and Bi having comparable masses dominate the low-frequency branches up to 4.5 THz. The Zr atom being lightest (mass=91.22 amu), contribute to the high-frequency atomic vibrations (above ~4.8 THz). Due to the comparable masses of Bi and Ir and their noticeable difference with Zr, there is a gap in between the acoustic and optic branches.

In ZrRhBi, The masses of Zr and Rh are comparable and lower than that of Bi, thus they contribute to the higher frequencies (>4 THz) whereas Bi being much heavier contributes to the lower frequencies (<3.5 THz). The large mass difference between these atoms causes even higher gap between the acoustic and optical branches. Due to this large mass difference, the $\kappa_L$ values are lower for ZrRhBi as compared to HfRhBi and ZrIrBi.

# References


1. M. Born and K. Huang, Dynamical theory of crystal lattices (Clarendon Press, 1954).
2. A. Reuss, Z. Agnew. Math. Mech.1929, **9**, 49.
3. W. Voight, Lehrbuch der Kristallphysik (Tubner, Leipzig, 1928).
4. Z. Hashin and S. Shtrikman, J. Mech. Phys. Solids 1962, **10**, 335 ; 1962, **10**, 343 .
5. Michael J. Mehl, Phys. Rev. B 1993, **47**, 2493 .
6. Hiroaki Muta, Takanori Kanemitsu, Ken Kurosaki, Shinsuke Yamanaka , Journal of Alloys and Compounds 2009, **469 ,** 50.
7. C. Yu, H. H. Xie, C. G. Fu, T. J. Zhu, X. B. Zhao, J. Mater. Res. 2012, **27**, 2457.
